# Supplementary material for: A New Algorithm for Non-stationary Contextual Bandits: Efficient, Optimal, and Parameter-free
Source: arXiv:1902.00980 source file (2019-06-18)
Supplement: Supplementary file 1 [file appendix-fictitious.tex]

\section{Bounding the overlap blocks and epochs}
\label{sec: repetitive block}

Define $\calE_i \triangleq [\tau_i,\min\{\tau_{i+1}-1,T\}]$ to be the entire interval of epoch $i$  and define $\calE_i'$ to be 
\begin{align*}
     \calE_i' \triangleq \calE_i\cup[\tau_i,\tau_i+2^{j^*}L-1]\quad j^*=\underset{j}{\mathrm{argmin}} ~ \tau_i+2^{j}L \ge \min\{T+1,\tau_{i+1}\}
\end{align*}
That is, $j^*$ is the last block on epoch $i$. Then we have the following observation:
\begin{lemma}\label{repeat_relation}
Suppose $i,i'$ are two epochs such that $i<i'$, and both $\calE_i'$ and $\calE_{i'}'$ contain $t$. Then we have $2(t-\tau_{i'})\le t-\tau_{i}$.
\end{lemma}
\begin{proof}
Let $j^*$ be the last block on epoch $i$. Because $|\calE_i'|=2^{j^*}=2\cdot 2^{j^*-1}\le 2|\calE_i|$,
we have $|\calE_i'|-|\calE_i|\le |\calE_i|$. Thus,
\begin{align*}
2(t-\tau_{i'})\le (t-\tau_{i'})+ |\calE_i'|-|\calE_i|\le (t-\tau_{i'})+|\calE_i|\le (t-\tau_{i'})+\tau_{i'}-\tau_{i}\le t-\tau_{i}
\end{align*}
\end{proof}
For any time $t$, let $n(t)$ be the number of $\calE_i'$ that contain $t$. Next lemma tries to bound $n(t)$:
\begin{lemma}
For any time $t$, we must have $n(t)\le\log_2(T)+2$.
\end{lemma}
\begin{proof}
Let $i_1<i_2<\cdots<i_{n(t)}$ be epochs such that $\calE_{i_k}'$ contains $t$ for any $k$. Applying Lemma~\ref{repeat_relation} recursively, we have
\begin{align*}
T\ge\left(t-\tau_{i_1}\right)\ge 2\left(t-\tau_{i_2}\right)\ge\cdots\ge 2^{n(t)-2}\left(t-\tau_{i_{n(t)-1}}\right)\ge 2^{n(t)-2}\ge 2^{n(t)-2}
\end{align*}
Taking logarithms on both sides completes the proof.
\end{proof}
Now we are ready to bound summation of regret over epochs:
\begin{lemma}
\begin{align*}
\sum_{i=1}^{S'}\sqrt{S_{\calE_i'}|\calE_i'|}=\otil(\sqrt{ST}),\quad \sum_{i=1}^{S'}\Delta_{\calE_i'}^{\frac{1}{3}}|\calE_i'|^{\frac{2}{3}}= \otil(\Delta^{\frac{1}{3}}T^{\frac{2}{3}})
\end{align*}
\end{lemma}
\begin{proof}
\begin{align*}
\sum_{i=1}^{S'}\sqrt{S_{\calE_i'}|\calE_i'|}\le \sqrt{\left(\sum_{i=1}^{S'}S_{\calE_i'}\right)\left(\sum_{i=1}^{S'}|\calE_i'|\right)}\le \sqrt{(\log_2(T)+2)S(2T)}
\end{align*}
Similarly, 
\begin{align*}
\sum_{i=1}^{S'}\Delta_{\calE_i'}^{\frac{1}{3}}|\calE_i'|^{\frac{2}{3}}\le \left(\sum_{i=1}^{S'}\Delta_{\calE_i'}\right)^{\frac{1}{3}}\left(\sum_{i=1}^{S'}|\calE_i'|\right)^{\frac{2}{3}}\le \left((\log_2(T)+2)\Delta\right)^{\frac{1}{3}}\left(2T\right)^{\frac{2}{3}}
\end{align*}
\end{proof}
